# Supplementary material for: Continuous-Depth Neural Models for Dynamic Graph Prediction
Source: arXiv:2106.11581 source file (2021-06-22)
Supplement: Supplementary file 1 [file appendix.tex]

\paragraph{Notation} 
We refer to the set of real numbers as $\R$. $\|\cdot\|_2$ is the norm induced by the inner product of $\R^n$. The origin of $\R^n$ is $\mathbbb{0}_n$. Scalars are denoted as lower--case letters, vectors as bold and lower--case and matrices as bold capital letters. Indices of arrays and matrices are reported as superscripts in round brackets. We use $s$ instead of $t$ as the depth variable to generalize the concept of \textit{time} to \textit{depth}. 
Throughout this paper the \textit{nested n--spheres} benchmark task introduced in \cite{dupont2019augmented} is used extensively. Namely, given $r>0$ define $\varphi: \R^n \to \mathbb{Z}$
\begin{equation}\label{benchmark}
    \varphi(\x) =
    \left\{
        \begin{matrix*}[l]
            -1 & \norm{\x}_2 < r\\
             1 & \norm{\x}_2 \geq r
        \end{matrix*}
    \right.~.
\end{equation}
We consider learning the map $\varphi(\x)$ with neural ODEs prepending a linear layer $\R^n \rightarrow \R$. Notice that $\varphi$ has been slightly modified with respect to \cite{dupont2019augmented}, to be \textit{well--defined} in its domain. For the one--dimensional case, we will often instead refer to map $\varphi(x) = -x$ as the \textit{crossing trajectories} problem. Unless otherwise stated, all ODEs are solved with the adaptive Dormand--Prince \cite{prince1981high} method available in the {\tt torchdiffeq} \cite{chen2018neural} PyTorch package. In nested $n$--spheres and crossing trajectories problems, we minimize \textit{mean squared error} (MSE) losses of model outputs and mapping $\varphi$. Additionally, for all experiments, complete information relative to the implementation is reported in the supplementary materials. The code will be open--sourced after the review phase and is included in the submission. 
\paragraph{Neural ODEs as universal approximators}
Vanilla neural ODEs are not, in general, universal function approximators (UFAs) \cite{zhang2019approximation}. Besides some recent works on the topic \cite{zhang2019approximation, li2019deep} this apparent limitation is still not well--understood in the context of continuous--depth models. When neural ODEs are employed as general--purpose black--box modules, some assurances on the approximation capabilities of the model are necessary. \cite{zhang2019approximation} noticed that a depth--invariant augmented neural ODE
\begin{equation}
    \begin{matrix*}[l]
    \dfrac{d}{ds}
    \begin{bmatrix}
        x\\
        a
    \end{bmatrix} =  
    \begin{bmatrix}
        \mathbb{0}_n\\
        f(x,\theta)
    \end{bmatrix}\\
    %%%
    \begin{bmatrix}
        x(0)\\
        a(0) 
    \end{bmatrix} = 
    \begin{bmatrix}
        u\\
        0
    \end{bmatrix}
    \end{matrix*},~~s\in[0,1]
\end{equation}
where the output is picked as $y := a(1)$, can approximate any function $\Psi:\R^d\rightarrow\R$ provided that the neural network $f(u,\theta)$ is an approximator of $\Psi$, since $a(1) = f(u,\theta)$, mimicking the mapping $u\mapsto f(u,\theta)$. Although this simple result is not sufficient to provide a constructive blueprint to the design of neural ODE models, it suggests the following (open) questions:
\begin{itemize}
    \item Why should we use a neural ODE if its vector field can solve the approximation problem as a standalone neural network?
    \item Can neural ODEs be UFAs  with non-UFA vector fields?
\end{itemize}
On the other hand, if neural ODEs are used in a \textit{scientific machine learning} context \cite{rackauckas2020universal} requiring an UFA neural network to parametrize the model provides it with the ability to approximate arbitrary dynamical systems.
